# Supplementary material for: RangeLDM: Fast Realistic LiDAR Point Cloud Generation
Source: arXiv:2403.10094 source file (2024-09-10)
Supplement: Supplementary file 1 [file X_suppl.tex]

\section{Visualization}
\label{sec:rationale}

\paragraph{Unconditional Generation Results.} 
We show more results compared with baselines on the KITTI-360~\cite{liao2022kitti} dataset in Figure~\ref{fig:sup_unconditional_kitti360}, where we supplemented the results of LiDAR VAE and LiDAR GAN. 
We see that the proposed method outperforms baselines and generates realistic structures with consistent LiDAR beams.
We also display the qualitative results compared with baselines on the nuScenes~\cite{caesar2020nuscenes} dataset in Figure~\ref{fig:sup_unconditional_nus}.

\begin{figure*}
    \centering
    \includegraphics[width=\linewidth]{imgs/sup_unconditional_kitti360.pdf}
    \caption{Qualitative results comparing against baselines for unconditional LiDAR generation on the KITTI-360 dataset. Real point clouds are only for reference. Our model produces results that closely resemble real-world data.}
    \label{fig:sup_unconditional_kitti360}
\end{figure*}

\begin{figure*}[h]
    \centering
    \includegraphics[width=\linewidth]{imgs/sup_unconditional_nus.pdf}
    \caption{Qualitative results comparing against baselines for unconditional LiDAR generation on the nuScenes dataset. Real point clouds are only for reference. The proposed method generates realistic point clouds with clear LiDAR scan lines while the baselines often generate noisy outputs.}
    \label{fig:sup_unconditional_nus}
\end{figure*}

\paragraph{LiDAR Point Cloud Upsampling.}

\begin{figure*}
    \centering
    \includegraphics[width=0.92\linewidth]{imgs/upsample_all.pdf}
    \caption{Comparison of point cloud upsampling results with more methods.}
    \label{fig:upsampling_all}
\end{figure*}

We present the visualization results of point cloud upsampling compared with more methods on KITTI-360, as shown in Figure~\ref{fig:upsampling_all}.
Bicubic and NN are classical upsampling methods, while PU-Net~\cite{yu2018pu}, DeepRS~\cite{chen2022deep}, and Grad-PU~\cite{Grad-PU} focus on point cloud upsampling. LiDARGen is a method specifically designed for LIDAR point clouds.
For PU-Net, DeepRS, and Grad-PU, the results shown were obtained by directly testing their pre-trained models. These methods were not retrained on our LIDAR dataset.

\paragraph{LiDAR Point Cloud Inpainting. }

We present more point cloud inpainting results compared with LiDARGen~\cite{zyrianov2022learning} on the KITTI-360 dataset in Figure~\ref{fig:sup_inpainting}, as a supplement to Figure~7. 
We observe that the proposed method recovers scenes with reasonable cars, roads, and walls, outperforming the competitive method.

\begin{figure*}
    \centering
    \includegraphics[width=\linewidth]{imgs/sup_inpainting.pdf}
    \caption{Qualitative results comparing against LiDARGen for LiDAR point cloud inpainting on the KITTI-360 dataset. We highlight the masked area with dashed blue boxes in the ground truth. \textbf{Blue}: inpainted area; \textbf{Red}: input point clouds.}
    \label{fig:sup_inpainting}
\end{figure*}

\paragraph{Visualization Results of Ablation Study. We compare the proposed method with different variants.}

Figure~\ref{fig:sup_ablation} displays the visualization results of all ablation variants in Section~5.4. 
It is evident that variant (a), which lacks Hough voting, captures the global structures but generates noisy point clouds. 
With Hough Voting and the range-guided discriminator, variants (b) and (c) significantly reduce noise. 
The red circles in (a), (b), and (c) highlight a discontinuity originating from the origin and pointing left in the point cloud.
In contrast, variant (d) mitigates the discontinuity using circular convolution but fails to accurately represent the scene's direction due to rotation variance. 
This issue is addressed in model (e) through the proposed direction conditional sampling.

\begin{figure*}
    \centering
    \includegraphics[width=\linewidth]{imgs/sup_ablation.pdf}
    \caption{Qualitative results of ablation study. }
    \label{fig:sup_ablation}
\end{figure*}

\paragraph{Conditioning the Model with Direction.} 

Figure~\ref{fig:sup_direction_conditional} shows the generation process under the condition of different directions (as described in Section~4.4. 
This demonstrates effective control over the direction of the generated point clouds.

\begin{figure*}
    \centering
    \includegraphics[width=\linewidth]{imgs/sup_direction_conditional.pdf}
    \caption{Demonstration of the sampling process of direction-conditional generation.}
    \label{fig:sup_direction_conditional}
\end{figure*}

\paragraph{Evaluation of cross dataset generalization (\textcolor{blue}{R4})}

We illustrate qualitative results for upsampling nuScenes data using our pretrained KITTI-360 upsampling model, as shown in Figure~\ref{fig:nus_up}, demonstrating the generalizability. More qualitative results will be included.

\begin{figure}[h]
  \centering
  % \fbox{\rule{0pt}{0.5in} \rule{0.9\linewidth}{0pt}}
  \includegraphics[width=0.9\linewidth]{imgs/nus2kitti360_upsample.pdf}
   \caption{NuScenes upsampling results.}
   \label{fig:nus_up}
\end{figure}

\section{Addition Ablation Studies}
\subsection{Additional analysis for the VQ regularizer}
Table~\ref{tab:ablation_vqvae} displays the reconstruction and generation performance of two regularizers. 
KL regularizers outperform VQ regularizers in both reconstruction and generation, despite similar convergence speeds (about 50k steps). 
This advantage may be due to the Gaussian distribution in the latent space aiding generalization.

\begin{table}[h]
\centering
\resizebox{0.40\linewidth}{!}{
\begin{tabular}{c|cccc}
\hline
Regularizer & $\text{PSNR}_\text{rec}$ $\uparrow$ & $\text{CD}_\text{rec}$ $\downarrow$ & $\text{MMD}_\text{gen}$ $\downarrow$\\
\hline
VQ &  $26.59$   & $0.1563$  & $9.57 \times 10^{-5}$ \\ 
KL & $\mathbf{27.19}$    & $\mathbf{0.0676}$  & $\mathbf{3.07 \times 10^{-5}}$ \\ 
\hline
\end{tabular}
} 
\caption{Ablation for regularizers. }
\label{tab:ablation_vqvae}
\end{table}
